# Supplementary material for: Dockerfile Flakiness: Characterization and Repair
Source: arXiv:2408.05379 source file (2025-02-11)
Supplement: Supplementary file 1 [file appendix.tex]

% !TEX root =  main.tex

\section{Appendix}
\label{sec:appendix}
